# Supplementary material for: Excited-state normal-modes analysis: the case of porphyrins
Source: arXiv:2307.04511 source file (2023-07-10)
Supplement: Supplementary file 1 [file SupportingInfo_porphyrin_arXiV.pdf]

# Excited-state normal-modes analysis: the case of porphyrins

Pavel Rukin, Deborah Prezzi,* and Carlo Andrea Rozzi*

*Cnr - Istituto Nanoscienze, via Campi 213/A, 41125 Modena (Italy)*

E-mail: deborah.prezzi@nano.cnr.it; carloandrea.rozzi@nano.cnr.it

## Supporting Information

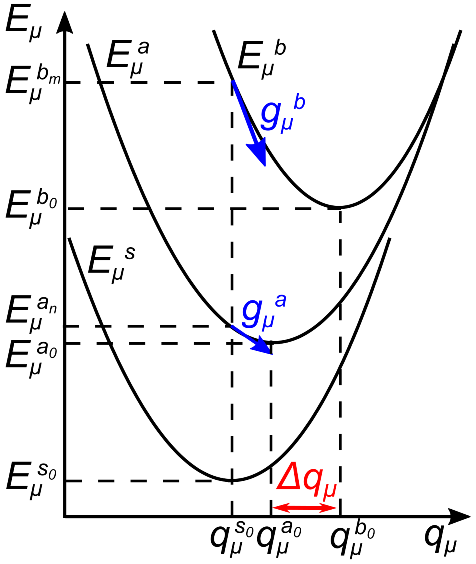


Figure S1: Definition of the shift $\Delta q_\mu$ along the mode $\mu$ in normal coordinates between initial state $a$ and final state $b$ when only the selected state can be optimized. $E_\mu^a$, $E_\mu^b$, $E_\mu^s$ are the PES along the mode $\mu$ of the defined states; $q_\mu^{a_0}$, $q_\mu^{b_0}$, $q_\mu^{s_0}$ and $E_\mu^{a_0}$, $E_\mu^{b_0}$,$E_\mu^{s_0}$ are the coordinates and energies of the initial, final, and selected states minima, respectively; $E_\mu^{a_n}$, $E_\mu^{b_m}$ are the energies at the vibrational states; $g_\mu^a$,$g_\mu^b$ are the gradients of $a$ and $b$ PES at the $q_\mu^s$ normal coordinate.

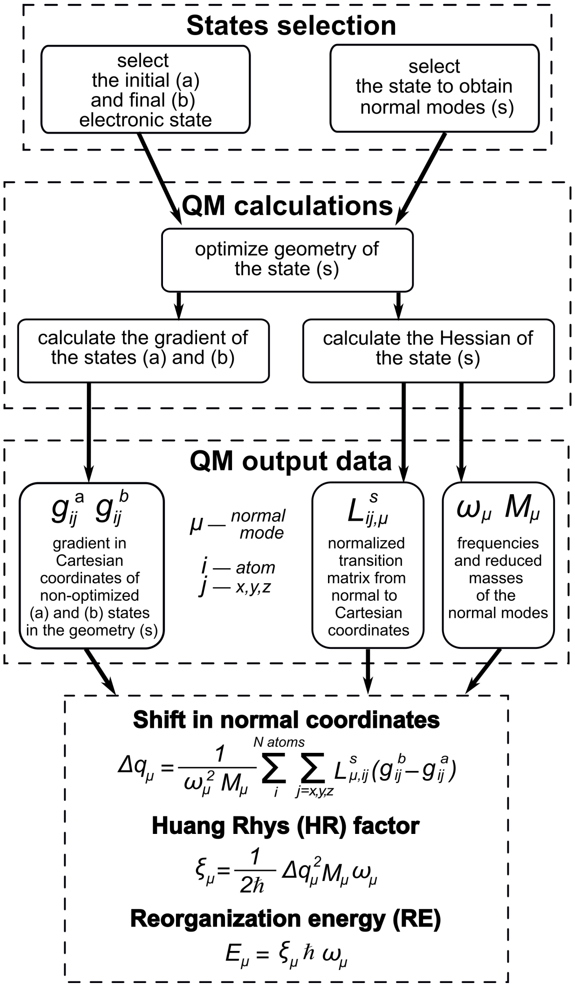


Figure S2: Flowchart of Huang Rhys (HR) and reorganisation energy (RE) calculations when the initial state $a$ cannot be optimized.

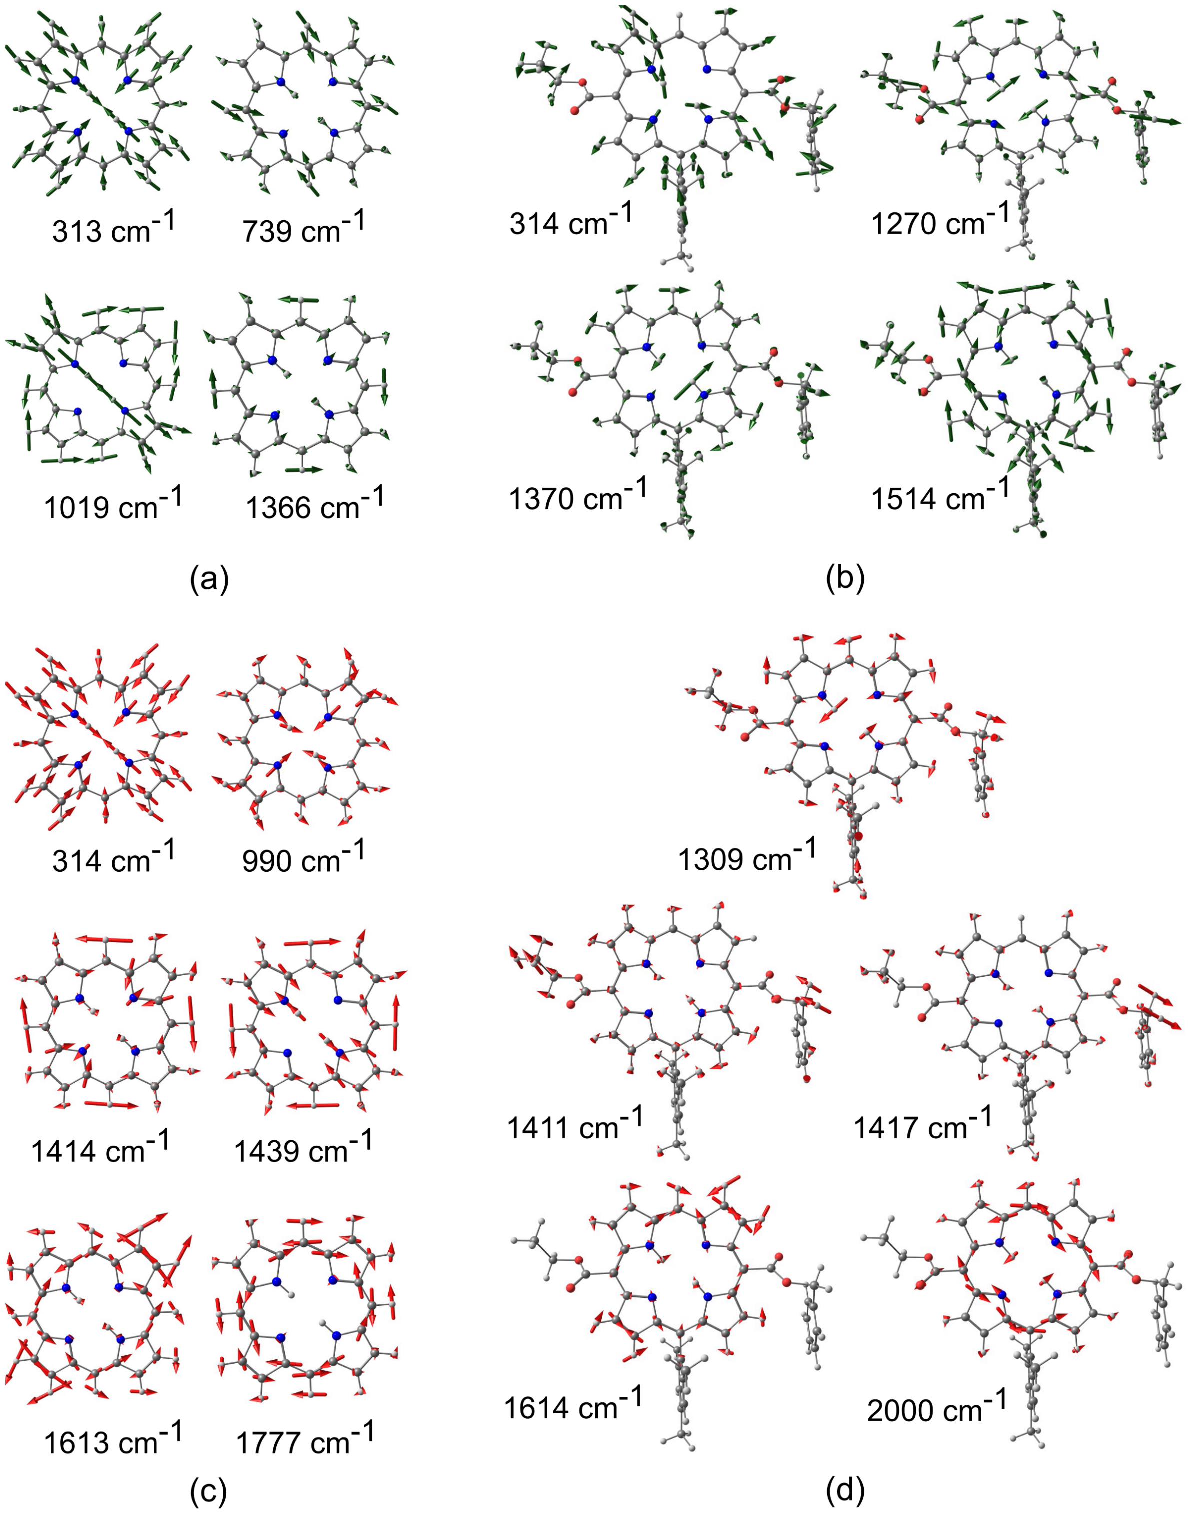


Figure S3: Atomic displacements of the modes with highest RE values for BP (a,c) and FP (b,d), considering both Q band ($S_0 \rightarrow S_1$ and $S_0 \rightarrow S_2$, panels a and b for BP and FP, respectively) and B band ($S_0 \rightarrow S_3$ and $S_0 \rightarrow S_4$, panels c and d for BP and FP, respectively).

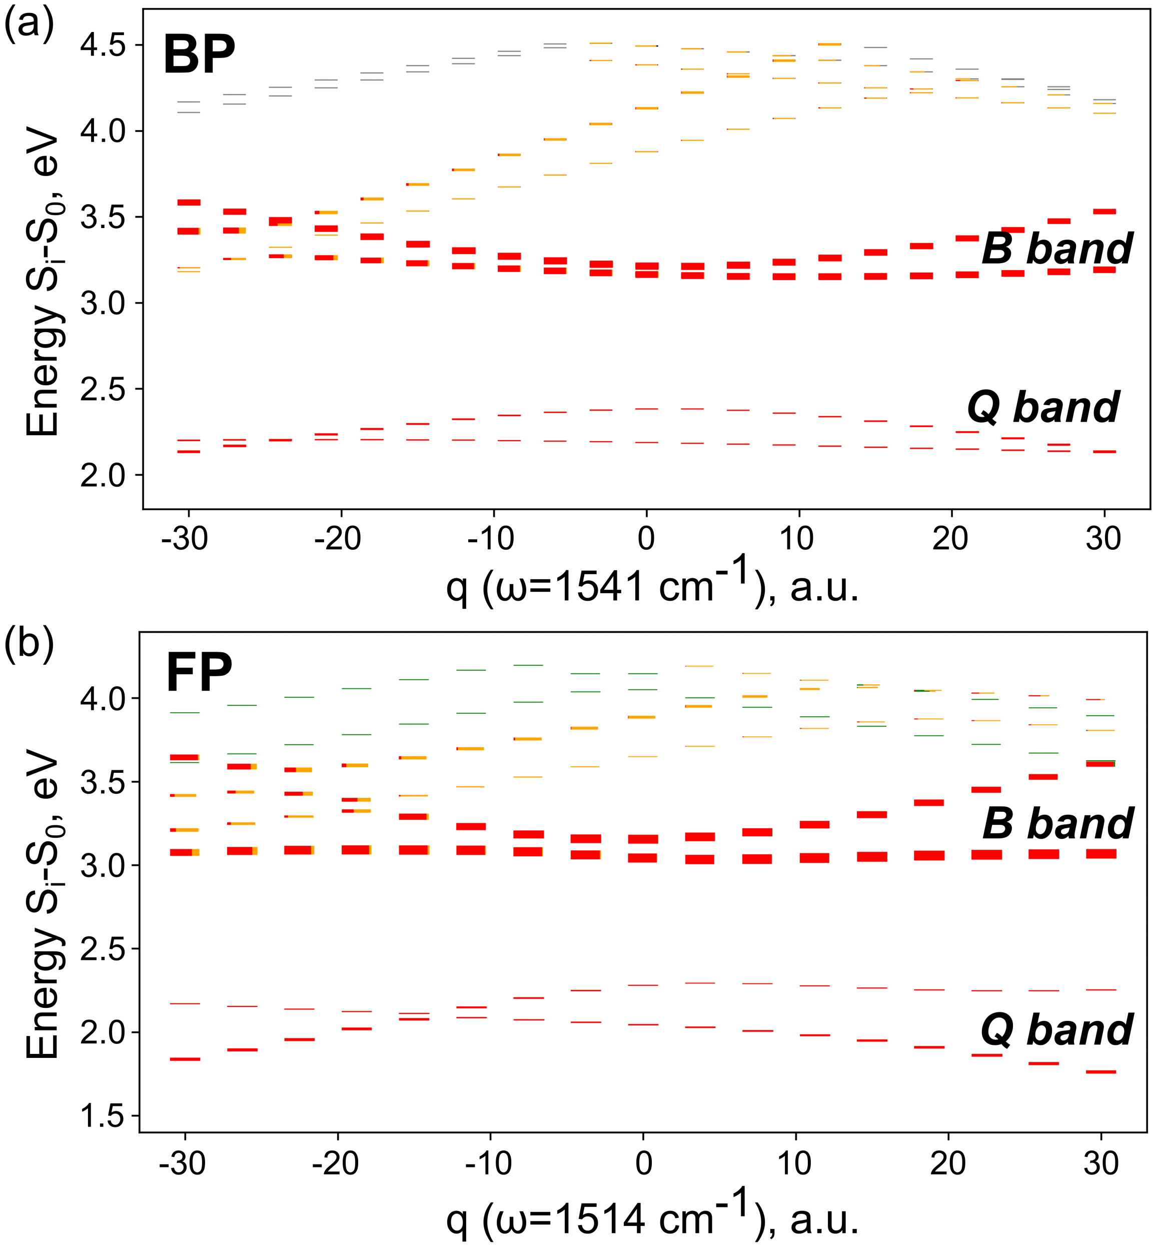


Figure S4: Trajectory scan along (a) the 1541 cm$^{-1}$ mode in BP and (b) the 1514 cm$^{-1}$ mode in FP. The colors indicate the orbital composition of the states based on Figure 7 of the main text. The line thickness is proportional to the oscillator strength of the transition (thick lines – bright states, thin lines – dark states). Energy values are shown with respect to $S_0$ at each normal coordinate ($E_{S_i} - E_{S_0}$).

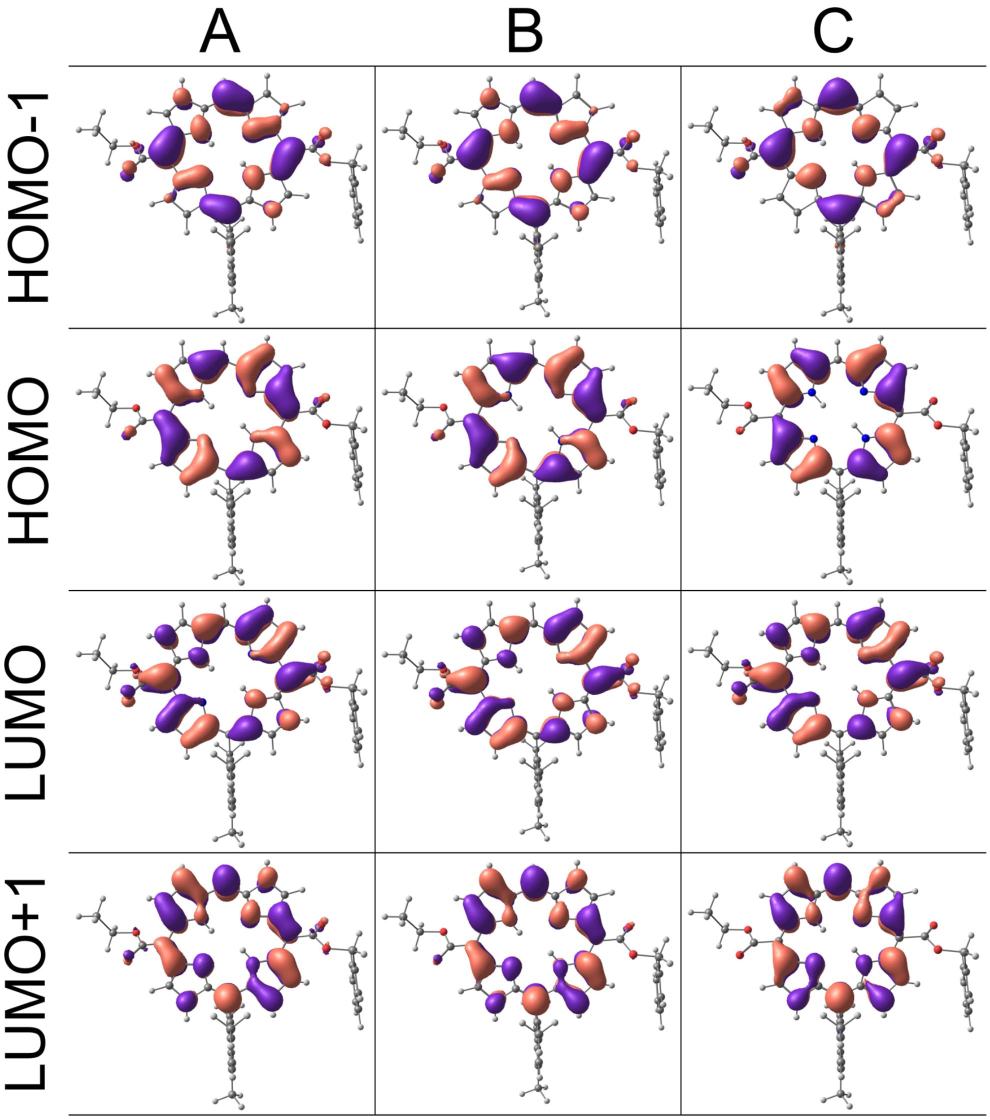


Figure S5: Molecular orbitals for the selected q points of the PES (A,B,C) analysed in Figure 8 of the main article.

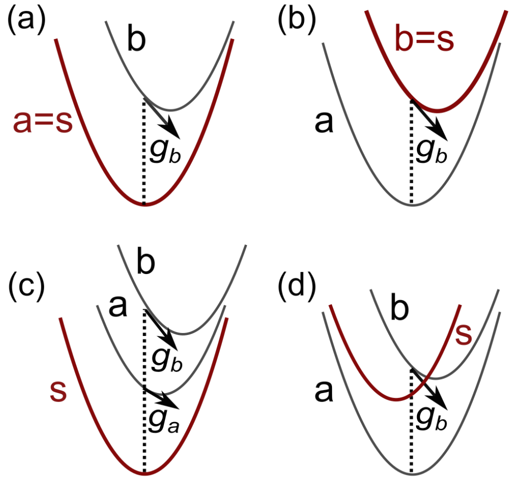


Figure S6: Possible choices for the selected $s$ state: (a) initial state $a$; (b) final state $b$; (c,d) a state that is different from both the initial and final states.
